# Supplementary material for: Physics of Laser-Wakefield Accelerators (LWFA)
Source: arXiv:2007.04622 source file (2020-07-09)
Supplement: Supplementary file 1 [file TXT_Appendix_LaserPlasma00.tex]

%\documentclass{DOC}

%\addbibresource{MyDissertation.bib}
%\usepackage[latin1]{inputenc}
%\usepackage[T1]{fontenc}
%\begin{document}
%\bibliographystyle{alpha}
%\titlespacing*{\section}{-2pt}{*0}{*0}
%\dominitoc% Initialization
%\tableofcontents

\cleardoubleoddemptypage
\chapter{Additional Derivations}
%\chapterimagelab{      textbox}
\chapterimageloc{Graphics/ChapterPics/test.pdf}
\section{Linear Plasma Waves}
\label{app:linear_plasma_waves}
The solution to a linear $3D$ plasma wave excited by a non-evolving laser pulse can be derived from the equation of motion, the continuity equation, and Poisson's equation. Written in the fluid description this set of equation is given by
\begin{align}
&\textbf{Equation of motion:} &\frac{\partial \vec{p}}{\partial t}=e \nabla\Phi+e \frac{\partial \vec{A}}{\partial t}-m_ec^2\nabla\gamma
%\frac{d \vec{p}}{d t}=\left(\frac{\partial }{\partial t} +\vec{v}\cdot \nabla \right)\vec{p}=-e[\vec{E}+\vec{v}\times\vec{B}] ,
\label{eq:eqofmotionA} %\label{eq:Lorentzplasma}
\\
&\textbf{Continuity equation:} &\frac{\partial n_e}{\partial t}+\nabla (n_e \vec{v})=0 ,
\label{eq:cont.eqA}
\\
&\textbf{Poisson's equation:} &\nabla^2 \Phi = -\frac{\rho}{\epsilon_0}=e\frac{\delta n_e}{\epsilon_0}, \label{eq:poissonA}
\end{align}
For the case of small laser intensities ($a_0 << 1$), the plasma density is only weakly perturbed $\delta n_e \ll n_{e,0}$ and the continuity equation \ref{eq:cont.eqA} can be written as
\begin{equation*}
\frac{\partial \delta n_e}{\partial t}+n_{e,0}\nabla\vec{v}=0.
\end{equation*} 
The above expression and the Poisson's equation (\ref{eq:poissonA}) can be now inserted in the derivative $\nabla$ of Eq.\ref{eq:eqofmotionA}. Keeping in mind $\nabla \vec{A}=0$ (Coulomb gauge) and $\vec{p}=m_e\vec{v}$ it follows for initially resting electrons at low intensities, i.e., $\gamma=1+a^2/2$
\begin{equation}
\left( \frac{\partial^2}{\partial t^2} + \omega_p^2 \right)\\
 \frac{\delta n_e}{n_{e,0}}=c^2\nabla^2 \frac{a^2}{2}. \label{eq:lincaseA}
\end{equation} 
This equation describes a forced oscillator, where the RHS represents the driving term. It is proportional to the ponderomotive force of the laser $F_{pond}=m_ec^2\nabla^2 a^2/2$. Expressed with the help of the Poisson's equation in terms of the scalar potential it yields in the moving frame coordinates ($\xi,\tau$)
\begin{equation}
\left( \frac{\partial^2}{\partial \xi^2} + k_p^2 \right)\phi
=k_p^2\frac{a^2}{2}. \label{eq:lincase2}
\end{equation}
Assuming a radial symmetry, an analytical solution of the inhomogeneous wave equation can be found in $3D$. It is given by \cite{Esarey1996, Gorbunov1987} 
\begin{equation*}
\phi(r,\xi)=-\frac{k_p}{4}\int_{\xi}^{\infty} a^2(r,\xi ')\sin(k_p(\xi-\xi')) \;\mathrm{d}\xi',
\end{equation*}
where 
%in the moving coordinate system $\phi(r,\xi=z-v_gt)$ 
$z$ is the propagation direction and $r\perp z$ the perpendicular direction.
For a Gaussian laser envelope $a=a_0\exp(-\xi^2/(c\tau_0)^2)\exp(-r^2/w_0^2)$, the solution of the integral for $\xi\rightarrow-\infty$, i.e., after the laser transit is given by \footnote{$\int_{-\infty}^{\infty}e^{-(x/c)^2}\sin(ax-b)\; \mathrm{d}x=-\sqrt{\pi}\vert c\vert e^{-(ac)^2/4}\sin(b)$}
\begin{equation}
\phi(r,\xi)=-a_0^2\sqrt{\frac{\pi}{2}}\frac{k_p}{4} c\tau_0\exp\left(-\frac{2r^2}{w_0^2}\right)\exp\left(-\frac{(k_p c \tau_0)^2}{8}\right)\sin(k_p\xi).
\end{equation}
Once the scalar potential $\phi$ is found, the electric field can be determined by its derivative and the electron density by the Poisson's equation:
\begin{align}
E_z=&-\frac{\partial \phi}{\partial \xi}=E_{p,0}f(r)\cos(k_p\xi), &
E_r=&-\frac{\partial \phi}{\partial r}=-E_{p,0}\frac{f(r)}{k_p}\frac{4r}{w_0^2}\sin(k_p\xi),\\
\frac{\delta n_e}{n_{e,0}}=&\frac{1}{k_p^2}\frac{\partial^2 \phi}{\partial \xi^2}=f(r)\sin(k_p\xi), &
f(r)=&a_0^2\sqrt{\frac{\pi}{2}}\frac{k_p}{4}  c\tau_0e^{-\frac{2r^2}{w_0^2}}e^{-\frac{(k_p c \tau_0)^2}{8}},
\end{align}
where $E_{p,0}$ corresponds to the cold fluid wave breaking field
$E_{p,0}=\frac{m_ec\omega_p}{e}$. % & E_{p,0}[\si{\giga\volt/m}]=96\sqrt{n_{e,0}[\SI{e18}{\per\cubic\cm}]}

\section{Non-linear Plasma Waves}
\label{app:nonlinear_plasma_waves}
For the $1D$ non-linear solution, the motion of electrons has to be decomposed into the propagation direction of the laser ($z$-direction) with the velocity $\vec{v_z}=c \vec{\beta_z}$ and the transverse direction in ($x$,$y$)-plane. The equation of motion in the transverse direction reads:
\begin{equation*}
\frac{d\vec{p_\perp}}{d t}=e(\vec{E_\perp}+\vec{v_z} \times \vec{B_\perp})=e \frac{d \vec{A_\perp}}{d t}  .
\end{equation*}
The longitudinal components of Eq.\ref{eq:Lorentz} and \ref{eq:energy_equation} can be subtracted from each other and -keeping in mind that the electromagnetic wave is a function of ($t-z$) only- results in 
\begin{equation*}
\frac{dE}{dt}-c\frac{dp_\parallel}{dt}=0.
\end{equation*}
An integration of both equation for an initially resting electron yields for the transverse and longitudinal momentum
\begin{align}
\vec{ p_\perp}=e\vec{A_\perp}\; \Leftrightarrow\; \vec{u_\perp}=\gamma \vec{\beta_\perp}=\vec{a}, \label{eq:vectorpotential_perpA}\\
E-cp_\parallel=m_ec^2\; \Leftrightarrow\; \gamma-1=u_\parallel.
\label{eq:vectorpotential_parallel}
\end{align}
As the vector potential $a_0$ only 
influences the electron velocity 
$\beta_\perp$ (Eq.\ref{eq:vectorpotential_perpA})
normal to the longitudinal component $\beta_\parallel$,
splitting the relativistic gamma factor $\gamma=\sqrt{1+u_\parallel^2+u_\perp^2}=1/\sqrt{1-\beta^2}$ in a $a_0$-dependent transverse part $\gamma_\perp$ and a longitudinal part $\gamma_\parallel$ is very convenient \citep{Esarey1996}.
It allows to rewrite the factor $\gamma$ with Eq.\ref{eq:vectorpotential_perpA} and Eq.\ref{eq:vectorpotential_parallel} in terms of the vector potential $a$:
\begin{align}
\gamma^2=&1+u_\perp^2+(\gamma-1)^2 & \Rightarrow& & \gamma=&1+\frac{a^2}{2},\\ \label{eq:gamma_in_plane_wave}
\gamma^2=&\frac{1+\gamma^2\beta_\perp^2}{1-\beta_\parallel^2}\equiv\gamma_\perp^2\gamma_\parallel^2 & \Rightarrow& & \gamma_\perp=&\sqrt{1+a^2}.
\end{align}
\\
In the longitudinal direction the term $\partial \vec{A}/\partial t$ in Eq.\ref{eq:eqofmotionA} can be ignored and the equation of motion is simplified in the laboratory and co-moving frame, respectively
\begin{align}
 \frac{1}{c}\frac{\partial u_z}{\partial t}=& \frac{\partial}{\partial z}(\phi-\gamma), &
\frac{1}{c} \frac{\partial u_z}{\partial \tau}=&\frac{\partial}{\partial \xi} \left(\phi-\gamma \left(1-\beta_p\beta_z\right)\right) .
\label{eq:z-motion_mod}
\end{align}
where $\beta_p=v_g/c$ the normalized plasma wave velocity. Analogous, the continuity equation \ref{eq:cont.eqA} and Poisson's equation \ref{eq:poissonA} can be written in the co-moving frame
\begin{align}
\frac{\partial}{\partial \tau}\frac{n_e}{ n_{e,0}} &=c\frac{\partial}{\partial \xi} \left( \frac{n_e}{n_{e,0}}\left( \beta_p-\beta_z \right) \right), &
\frac{\partial^2 \phi}{\partial \xi^2}=k_p^2\left(\frac{n_e}{n_{e,0}}-1\right).
 \label{eq:conteq_mod}
\end{align}
The set of equation expressed in the co-moving coordinates can be now applied to the quasi-static approximation, under the assumption that the laser pulse envelope does not evolve significantly during the transit time of the laser. This allows effectively neglect the partial derivative $\partial / \partial \tau $ relative to $\partial/\partial \xi$ in $\xi$ and %Eq.\ref{eq:partial_derivative}.
Eqs. \ref{eq:z-motion_mod} and \ref{eq:conteq_mod} can be integrated considering the integration constant in the absence of the plasma wave, i.e., before the arrival of the pulse $\xi \rightarrow \infty$
\begin{align}
\begin{split}
\frac{n_e}{n_{e,0}} \left( \beta_p - \beta_z\right)&=const. \;\;\;\;\;\;\;\;\;\;\;\; \xRightarrow[]{n\left(\xi=\infty\right)=1} \;\;\;\;\;\;\;\;\;\;\;\; \frac{n_{e}}{n_{e,0}}= \frac{\beta_p}{\beta_p-\beta_z},\\
\phi-\gamma \left(1-\beta_p\beta_z \right)&=const. \;\;\;\;\;\;\;\;\;\;\;\; \xRightarrow[\beta_z\left(\xi=\infty\right)=0]{\Phi=0,\gamma=1} \text{		} \phi+1=\gamma\left(1-\beta_p\beta_z\right).
\end{split}
\label{eq:cont_eq_comoving}
\end{align}
Rearranging these expressions to the following explicit form \citep{Gibbon2005}
\begin{align*}
\gamma&=\gamma_p^2\left(1+\phi\right)\left(1-\beta_p\Psi\right), &\beta_z&=\frac{\beta_p-\Psi}{1-\beta_p\Psi} 
& \text{with     } \Psi&=\left(1-\frac{1+a^2}{\gamma_p^2\left(1+\phi\right)^2}\right)^{1/2}
\end{align*}
allows to eliminate $\beta_z$ in Eq.\ref{eq:cont_eq_comoving}, which results in
\begin{equation*}
\frac{n_e}{n_{e,0}}=\gamma_p^2\beta_p\left(\frac{1}{\Psi}-\beta_p \right)
\end{equation*}
Finally, inserting the above expression in the Poisson's equation (Eq.\ref{eq:conteq_mod}) yields the wake potential in the co-moving coordinates for arbitrary pump strength
\begin{equation}
\frac{\partial^2 \phi}{\partial \xi^2}=k_p^2\gamma_p^2\left(\beta_p\left(1-\frac{1+a^2}{\gamma_p^2\left(1+\phi\right)^2}\right)^{-\sfrac{1}{2}}-1\right).
\end{equation}
This non-linear ordinary differential equation can now be solved for any desired laser pulse shapes $a(\xi)$ numerically. 

%%\bibliography{MyDissertation}
%
%%%\printbibliography
%%%\end{document}
